# Supplementary material for: FlairGPT: Repurposing LLMs for Interior Designs
Source: arXiv:2501.04648 source file (2025-08-30)
Supplement: Supplementary file 1 [file BlankConstraints.pdf]

# 1 Blank Constraint Cost Functions for Individual Constraints

---

```
1 from Class_Structures import *
2 from shapely.geometry import Polygon
3
4 ### Throughout, the sides of the objects are defined as follows:
5 # 'back' of the object would be the headboard of a bed, or the back of a chair
6 # 'front' of the object would be the foot of a bed, or the front of a wardrobe (the side with the doors)
7 # 'left' would be the left side of the object, when standing behind it
8 # 'right' would be the right side of the object, when standing behind it
9
10 def ind_next_to_wall(positions, room, object_index):
11     """ This function ensures an object is next to a wall in a room. Specifically the back of the object.
12     Example constraint: "The tv should be against a wall."
13
14     Args:
15     positions: list of floats, x, y, theta values for all objects in the room
16     room: rectangular Room object
17     object_index: int, index of the object in the room's object list)
18
19     """
20
21     return
22
23
24 def ind_near_wall(positions, room, object_index, side = 'back', max_dist = 0.5):
25     """ This function ensures an object is near to a wall in a room (within a specific distance, NOT next to).
26     The specific side of the object will be used. If no side is given, the back of the object will be used.
27
28     Args:
29     positions: list of floats, x, y, theta values for all objects in the room
30     room: rectangular Room object
31     object_index: int, index of the object in the room's object list
32     side: string, one of 'back', 'front', 'left', 'right' defines which side of the object to check e.g back of bed
33     max_dist: float, maximum distance the object should be from the wall
34
35     """
36
37     return
38
39 def ind_close_to_fixed_object(positions, room, object_index, fixed_object_type, side = None, max_dist = 0.5):
40     """ The function ind_close_to_fixed_object is used for 3 purposes:
41     1) an object should be next to a window (fixed_object_type = 'window')
42     2) an object should be next to a door (fixed_object_type = 'door')
43     3) an object should be next a socket (fixed_object_type = 'socket')
44
45     If side is given, the specific side of the object will be used.
46
47     Args:
48     positions: list of floats, x, y, theta values for all objects in the room
49     room: rectangular Room object
50     object_index: int, index of the object in the room's object list
51     fixed_object_type: string, type of fixed object to check. One of 'window', 'door', 'socket'
52     side: string, one of 'back' (for things like headboard of bed, or back of bookshelf), 'front'
53     (for things like foot of bed or front of bookshelf), 'left', 'right', defines which side of the object to check
54     e.g back of bed
55     max_dist: float, maximum distance between the object and the fixed object to be considered close to it.
56     Write this as a float e.g. 2.0.
57
58     """
59
60     return
61
62 def ind_away_from_fixed_object(positions, room, object_index, fixed_object_type, min_dist = 2.0):
63     """ This function is used for 3 purposes:
64     1) an object should be away from a window (fixed_object_type = 'window')
```

```

64         2) an object should be away from a door (fixed_object_type = 'door')
65         3) an object should be away from a socket (fixed_object_type = 'socket')
66
67     Args:
68     positions: list of floats, x, y, theta values for all objects in the room
69     room: rectangular Room object
70     object_index: int, index of the object in the room's object list
71     fixed_object_type: string, type of fixed object to check. One of 'window', 'door', 'socket'
72     min_dist: float, minimum distance between the object and the fixed object to be considered away from it.
73     Write this as a float, e.g. 2.0.
74     """
75
76     return
77
78 def ind_accessible(positions, room, object_index, sides, min_dist = None):
79     """ This function ensures that an object is accessible from given sides. It can also ensure that
80     there is nothing too close to a given side of an object (e.g. if there needs to be clearance around something).
81     If no sides are given, the front side is used. If min_dist is given, then this function
82     will act as a clearance constraint. If you want all the sides to be accessible,
83     sides = ['front', 'back', 'left', 'right'].
84
85     Args:
86     positions: list of floats, x, y, theta values for all objects in the room
87     room: rectangular Room object
88     object_index: int, index of the object in the room's object list
89     sides: a list of strings, each one one of 'front', 'left', 'right', defines which side of the object to check
90     min_dist: float (optional), minimum distance clearance for the object on the sides given.
91     Write this as a float, e.g. 1.0.
92     """
93
94     return
95
96 def ind_central(positions, room, object_index, both = False):
97     """ This function ensures that an object is centrally placed in the room.
98
99     Args:
100     positions: list of floats, x, y, theta values for all objects in the room
101     room: rectangular Room object
102     object_index: int, index of the object in the room's object list
103     both: bool (optional), if True, then the object should be placed centrally in both x and y. For example for a bed,
104           but for a dining table, it should be True.
105     """
106
107     return
108
109 def ind_not_block_fixed_object(positions, room, object_index, fixed_object_type):
110
111     """ This function is used for 2 purposes:
112         1) an object does not block a window (fixed_object_type = 'window')
113         2) an object does not block a door (fixed_object_type = 'door')
114
115     Args:
116     positions: list of floats, x, y, theta values for all objects in the room
117     room: rectangular Room object
118     object_index: int, index of the object in the room's object list
119     fixed_object_type: string, type of fixed object to check. E.g one of 'window', 'door', 'plug'
120     """
121
122     return
123
124 def ind_under_window(positions, room, object_index):
125
126     """ This function ensures that the object will be placed underneath a window.
127     For example, you might want a desk or a dresser below (but not blocking) a window. You would NOT use this for any
128     objects that would be tall, for example a wardrobe or a fridge. Example constraint "The desk should be under
129     the window", "The desk should look out the window". Don't use with ind_not_block_fixed_object for a window

```

```

130         and the same object.
131
132     Args:
133     positions: list of floats, x, y, theta values for all objects in the room
134     room: rectangular Room object
135     """
136
137     return
138
139 def ind_facing_into_room(positions, room, object_index):
140     """ ind_facing_into_room is a function that ensures and object faces into the center of the room.
141     E.g. an armchair might face into the room.
142
143     Args:
144     positions: list of floats, x, y, theta values for all objects in the room
145     room: rectangular Room object
146     object_index: int, index of the object in the room's object list
147
148     """
149     return
150
151 def ind_in_region(positions, room, object_index, region_name, weight = 5.0):
152     """ This function ensures that an object is in a given region. This should NOT be used with the
153     optimize_primary_objects function.
154
155     Args:
156     positions: list of floats, x, y, theta values for all objects in the room
157     room: rectangular Room object
158     object_index: int, index of the object in the room's object list
159     region_name: string, name of the region for the object to be in
160     weight: float, weight of the constraint
161     """
162
163     return
164
165
166 def ind_not_against_wall(positions, room, object_index, min_dist = 0.5):
167
168     """ ind_not_against_wall is a function that ensures an object is not against a wall.
169     For example "the rug should not be touching the wall" or "the dining table should not be against the wall".
170
171     Args:
172     positions: list of floats, x, y, theta values for all objects in the room
173     room: rectangular Room object
174     object_index: int, index of the object in the room's object list
175     min_dist: float, minimum distance the object should be from the wall. Please write this as a float, e.g. 2.0.
176     """
177
178     return
179
180 def ind_in_corner(positions, room, object_index, side = 'back', max_dist = 0.5):
181     """ This function can be used to ensure that an object is placed into a corner.
182     The back of the object will always be placed closest to the corner.
183
184     Args:
185     positions: list of floats, x, y, theta values for all objects in the room
186     room: rectangular Room object
187     object_index: int, index of the object in the room's object list
188     max_dist: float, maximum distance the object should be from the wall
189     """
190     return

```

---

## 2 Blank Constraint Cost Functions for Inter-Object Constraints

---

```
1
2 import numpy as np
3 from Class_Structures import *
4 from shapely.geometry import Polygon
5
6 ### Throughout, the sides of the objects are defined as follows:
7 # 'top' or 'back' of the object would be the headboard of a bed, or the back of a chair
8 # 'front' or 'bottom' of the object would be the foot of a bed, or the front of a wardrobe (the side with the doors)
9 # 'left' would be the left side of the object, when standing behind it
10 # 'right' would be the right side of the object, when standing behind it
11
12
13 def io_next_to(positions, room, object1_index, object2_index, side1 = None, side2 = None):
14     ##DO NOT USE THIS WITH io_surround, IT WILL BE REDUNDANT OR CONTRADICTIONARY.
15     """ This function ensures that two objects are next to each other in a room.
16         This should only be used when necessary e.g. for nightstands and a bed, or a desk and desk chair.
17         This should not be used for dining chairs around a table or similar relationship, for that use io_surround.
18         If side1 is given, the specific side of object1 will be used. If side2 is given,
19         the specific side of object2 will be used. E.g. the 'front' of the chair should be next to the 'front' of the desk.
20         If no side is given, then any of the sides will be used.
21
22     Args:
23     room: rectangular Room object
24     object1: Object object
25     object2: Object object
26     side1: string, one of 'top' or 'back', 'bottom' or 'front', 'left', 'right', defines which side of object1 to use
27     side2: string, one of 'top' or 'back', 'bottom' or 'front', 'left', 'right', defines which side of object2 to use
28     """
29     return
30
31 def io_away_from(positions, room, object1_index, object2_index, min_dist = 2.0):
32     """ This function ensures that two objects are away from each other in a room.
33         For example, a bed should be away from a desk.
34
35     Args:
36     positions: list of floats, x, y, theta values for all objects in the room
37     room: rectangular Room object
38     object1_index: int, index of object1 in the room
39     object2_index: int, index of object2 in the room
40     min_dist: float, minimum distance between the two objects. Please write this as a float, e.g. 2.0.
41
42     """
43     return
44
45 def io_near(positions, room, object1_index, object2_index, max_dist = 3.0):
46     """ This function ensures that two objects are within a certain distance to each other.
47         They are not necessarily next to each other, but they are close. This might be for a bookshelf
48         and an armchair, or a mirror and a wardrobe.
49
50     Args:
51     room: rectangular Room object
52     object1_index: Object object
53     object2_index: Object object
54     max_dist: furthest distance between the two objects. Please write this as a float, e.g. 3.0.
55
56     """
57     return
58
59 def io_parallel(positions, room, object1_index, object2_index, center_object_info = None, max_dist = 2.0):
60     """ This function ensures that two objects have the same orientation in a room.
61         That is, that they are parallel to each other. It does not handle distance, so if
62         proximity is important, please combine this function with io_near, or io_next to, or even io_between.
63
64     """
```

```

64     Args:
65     positions: list of floats, x, y, theta values for all objects in the room
66     room: rectangular Room object
67     object1_index: int, index of object1 in the room
68     object2_index: int, index of object2 in the room
69     """
70     return
71
72 def io_facing(positions, room, object1_index, object2_index, both = False):
73     """ This function ensures that object1 is facing object2 in a room.
74     If both is True, then object2 will also be facing object1.
75     For example, a sofa and tv should face each other, so in that instance both would be True.
76
77     Args:
78     positions: list of floats, x, y, theta values for all objects in the room
79     room: rectangular Room object
80     object1_index: int, index of object1 in the room
81     object2_index: int, index of object2 in the room
82     both: bool, if True, object2 will also be facing object1
83     """
84     return
85
86 def io_infront(positions, room, object1_index, object2_index, dist = 0.8, parallel = False):
87     """ This function ensures that object1 is in front of object2 (both moving_objects i.e. not windows or doors).
88     E.g a coffee table should be in front of a sofa.
89
90     Args:
91     positions: list of floats, x, y, theta values for all objects in the room
92     room: rectangular Room object
93     object1_index: int, Object object
94     object2_index: int, Object object
95     dist: float, desired distance between two objects. E.g. if its a sofa and a coffee table, the distance should
96     be around 0.8m, if its a sofa and a fireplace, the distance should be around 2m/2.5m.
97     parallel: bool, if True, object1 will be parallel to object2. This would be used for a coffee table in front
98     of a sofa, but not for a sofa in front of a fireplace.
99     """
100
101     return
102
103 def io_perp(positions, room, object1_index, object2_index, center_object_index = None):
104     """ This function ensures that two objects are aligned in a room perpendicularly.
105     If center is given, the objects will be aligned about that point. For example, a sofa and chair might be aligned
106     perpendicularly about a coffee table or a side table.
107
108     Args:
109
110     positions: list of floats, x, y, theta values for all objects in the room
111     room: rectangular Room object
112     object1_index: int, index of object1 in the room
113     object2_index: int, index of object2 in the room
114     center_object_index: int, index of object in room.moving_objects to be used as the pivot for the alignment
115     (e.g. a coffee table or a table)
116     """
117
118     return
119
120 def io_surround(positions, room, central_object_index, object_indices):
121     ## IF YOU USE THIS FUNCTON, DO NOT ALSO USE "IO_NEXT_TO" AS IT WILL BE REDUNDANT OR CONTRADICTIONARY.
122     """ This function ensures that central_object is surrounded by all the objects in object_indices.
123     This would be used for chairs around a dining table. This should NOT be combined with io_next_to,
124     as that would be redundant or
125     it would contradict.
126
127     Args:
128     positions: list of floats, x, y, theta values for all objects in the room
129     room: rectangular Room object

```

```

130         central_object_index: int, Object object
131         object_indices: list of ints, indices of Object objects
132     """
133
134     return
135
136 def io_not_facing(positions, room, object1_index, object2_index):
137     """ This function ensures that object1 is NOT facing object2 in a room.
138         For example, a bed should not face a mirror.
139         Args:
140         positions: list of floats, x, y, theta values for all objects in the room
141         room: rectangular Room object
142         object1_index: int, index of object1 in the room
143         object2_index: int, index of object2 in the room
144     """
145     return
146
147 def io_between(positions, room, object1_index, object2_index, object3_index):
148     """ This function ensures that object1 is in between the two objects object2 and object3.
149         This would be used for something like a side table being between two chairs, or maybe a bed being
150         between two nightstands. Or a nightstand going between two beds.
151
152         Args:
153         positions: list of floats, x, y, theta values for all objects in the room
154         room: rectangular Room object
155         object1_index: int, index of object1 in the room (** this is the object that will go
156         in between the other two objects)
157         object2_index: int, index of object2 in the room
158         object3_index: int, index of object3 in the room
159     """
160     return
161

```

---

### 3 Blank Constraint Cost Functions for Tertiary Constraints

```

1  ## All the Individual Object constraint functions are defined here
2  from Class_Structures import *
3  from shapely.geometry import Polygon, Point
4  from shapely import distance
5  from Individual import *
6  from Setup_Functions import *
7  from Global import *
8  from scipy.optimize import minimize
9
10
11 def rug_under_central(positions, room, rug_index, object_index):
12
13     """ This function ensures that the rug is placed under the central object.
14
15     Args:
16     positions: list of floats, x, y, theta values for all objects in the room
17     room: rectangular Room object
18     rug_index: int, index of the rug object in the room.tertiary_objects list
19     object_index: int, index of the central object in the room.moving_objects list
20     """
21
22     return
23
24 def rug_under_central_forward(positions, room, rug_index, object_index):
25
26     """ This function ensures that the rug is placed under the central object, oriented correctly,
27     and moved slightly forward. E.g. this would be used for a rug that is placed under a bed.
28

```

```

29     Args:
30     positions: list of floats, x, y, theta values for all objects in the room
31     room: rectangular Room object
32     rug_index: int, index of the rug object in the room.tertiary_objects list
33     object_index: int, index of the central object in the room.moving_objects list
34     """
35     return
36
37 def on_top_central(positions, room, tertiary_index, other_index):
38
39     """ This function ensures that the tertiary object is placed on top of the central object.
40     This would be used for placing a table lamp on top of a nightstand, for example.
41
42     Args:
43     positions: list of floats, x, y, theta values for all objects in the room
44     room: rectangular Room object
45     tertiary_index: int, index of the tertiary object in the room.tertiary_objects list
46     other_index: int, index of the central object in the room.moving_objects list
47     """
48     return
49
50 def on_top_corner(positions, room, tertiary_index, other_index, corner = 'tl'):
51
52     """ This function ensures that the tertiary object is placed on top of the central object, at a specific corner.
53     This would be used for placing a lamp on the top left corner of a desk, for example.
54
55     Args:
56     positions: list of floats, x, y, theta values for all objects in the room
57     room: rectangular Room object
58     tertiary_index: int, index of the tertiary object in the room.tertiary_objects list
59     other_index: int, index of the central object in the room.moving_objects list
60     corner: str, corner of the central object where the tertiary object should be placed.
61     Options are 'tl', 'tr', 'bl', 'br'
62     """
63
64     return
65
66 def on_wall_near(positions, room, tertiary_index, other_index):
67
68     """ This function ensures that the tertiary object is placed on the wall near the central object.
69     This would be used for placing a painting on the wall near a dining table, for example.
70
71     Args:
72     positions: list of floats, x, y, theta values for all objects in the room
73     room: rectangular Room object
74     tertiary_index: int, index of the tertiary object in the room.tertiary_objects list
75     other_index: int, index of the central object in the room.moving_objects list
76     """
77
78     return
79
80 def on_wall_in_region(positions, room, tertiary_index, region_name):
81
82     """ This function is used to place a tertiary object on the wall in a specific region of the room.
83     This would be used for placing a painting on the wall in the living region, for example.
84
85     Args:
86     positions: list of floats, x, y, theta values for all objects in the room
87     room: rectangular Room object
88     tertiary_index: int, index of the tertiary object in the room.tertiary_objects list
89     region_name: str, name of the region where the tertiary object should be placed
90     (e.g. 'living', 'dining', 'bedroom')
91     """
92     return
93
94 def center_ceiling(positions, room, tertiary_index):

```

```

95     """ This function ensures that the tertiary object is placed in the center of the ceiling.
96     This would be used for placing a chandelier/ceiling light in the center of the room.
97
98     Args:
99     positions: list of floats, x, y, theta values for all objects in the room
100    room: rectangular Room object
101    tertiary_index: int, index of the tertiary object in the room.tertiary_objects list
102    """
103    return
104
105 def ceiling_above(positions, room, tertiary_index, other_index):
106     """ This function ensures that the tertiary object is placed on the ceiling above the central object.
107     This would be used for placing a ceiling fan above a bed, or a chandelier above a dining table for example.
108
109     Args:
110     positions: list of floats, x, y, theta values for all objects in the room
111     room: rectangular Room object
112     tertiary_index: int, index of the tertiary object in the room.tertiary_objects list
113     other_index: int, index of the central object in the room.moving_objects list
114     """
115     return
116

```

---
