# Supplementary material for: FlairGPT: Repurposing LLMs for Interior Designs
Source: arXiv:2501.04648 source file (2025-08-30)
Supplement: Supplementary file 2 [file fulloutput.pdf]

# Input: “A bedroom that is 4m x 5m.”

## Extracting Parameters

**Prompt 1:** I am designing the layout for a bedroom that is 4m x 5m. Give me the dimensions of the room, as well as the number of windows, doors, and sockets. For each of these, tell me the dimensions in meters, which wall it should be on, as well as where on the wall it should be (a value between 0 and 1 determining how far along the wall it should be). Here is an example for a room and window set up:

{Room: width = 5, length = 6}, {Object type: window, width = 1, length = 0.1, wall = south, position = 3}. The windows and doors should all have length 0.1. Ensure that every object has dimensions, position, and wall. No other text please. Just the list with no commentary or explanation.

**Prompt 2**: The functions in the following file are used to create a room and out objects in it: + file_contents1. The room is described as “a bedroom that is 4m x 5m”. For every element in this list, fixed_objects, translate it into a function call using the file attached.

For example, given the room descriptor 'a small kitchen' as well as the list: {Room: width = 5, length = 6}, {Object type: window, Number: 1, width = 1, length = 0.1, wall = south, position = 0.3}, the output would be:

kitchen = create_room(5, 6), create_fixed_object(kitchen, 'window', 1, 0.1, 'south', position = 0.3). Return only the python script.

No other text. Please ensure the correct number of inputs are given for each function.

**Output 1:**

```
room = create_room(4, 5)
create_fixed_object(room, 'door', 0.9, 0.1, 'west', 0.1)

create_fixed_object(room, 'window', 1.2, 0.1, 'south', 0.4)

create_fixed_object(room, 'window', 1.2, 0.1, 'east', 0.6)

create_fixed_object(room, 'socket', 0.2, 0.1, 'north', 0.3)

create_fixed_object(room, 'socket', 0.2, 0.1, 'west', 0.5)

create_fixed_object(room, 'socket', 0.2, 0.1, 'east', 0.2)
```

## Regions

**Prompt1**: I am designing the layout of a “a bedroom that is 4m x 5m”, that is 4m x 5m. Interior designers suggest that a good layout will have different regions in the room for different functions. What regions should I use, and how many regions (minimum is 1 region - small rooms, e.g. 3x3, 2x3, etc, should only have 1 region, small medium sized rooms will have 2, 3x4, 4x3, 4x4, medium will have 3, etc) should there be based on the description, as

well as the size of the room. Make sure to not add too many regions as this causes overcrowding (very few rooms will have more than 4 regions). Return this as a simple bullet list of regions to include. Return these in list of priority order. Do NOT add too many regions. Only return the list of regions. No other information please.

**Output**: ['sleeping', 'storage', 'work']

**Prompt 2:** Given the room name: room_name , and the regions: regions, using the function region_setup defined below, initialise each region. For example 'eating region' might output 'region_setup(kitchen, 'eating', 0). Where possible the region name ('eating') should be only one word. No other text please, only the python script. Don't include the function in the output. The function is:

```
def region_setup(room_name, name, index):
   '''A function that initialises the regions in a room randomly.
      Inputs:
      room_name: Room obj (this should be the name of the room)
      name: str, the name of the region e.g 'sleeping'index: int, the index of the region (0, 1, 2,
...). First one must be 0, and the rest must be in order.
   '''
   return
```

# Primary Objects, Secondary Objects

**Prompt 1:** The room is described as "a bedroom that is 4m x 5m". Now for each one of the regions: regions, what is the most important object to include (keep in mind the room description), and what are its dimensions (give width of back of object and length of side of object but not height) in meters. ONLY one object per region. Don't include any objects that go on the walls, e.g. wall art, and don't include any rugs/mats. The size of the room is 4m x 5m, bear this in mind when choosing the objects and the size of the objects (i.e. put small objects in small rooms). Give no other information please.

**Output:**
- Sleeping: Bed, 1.5m x 2m
- Storage: Wardrobe, 1.2m x 0.6m
- Work: Desk, 1.2m x 0.6m

**Prompt 2:** Given a room described as: "a bedroom that is 4m x 5m", with size: 4m x 5m with these regions within it: regions, and these primary objects already in it: primary_objects, what other objects should be added in?
Give me 0-4 objects per region (depending on the size of the room - fewer objects for smaller rooms, and more objects for larger room) that should be added into the room (so make sure they are the most appropriate/necessary objects for their regions). Ensure to add objects that are necessary,e.g. if there's a desk, always add a desk chair. Try not to give objects that are redundant, e.g. if there is a tv stand in the room, you don't need a media console. Objects should be things like furniture or plants or other objects that sit on the floor.For each one,

make sure that they make sense to go into one of the regions, and tell me which region they should go into. There can be more than one of each object kind (eg. multiple dining chairs or multiple nightstands) so make sure to specify how many of each object. Make sure to also give the dimensions of every object in meters (width of the back of the object and length of the side of the object but NOT HEIGHT). Remove any objects that are not placed directly on the floor, e.g. table lamp, and remove any objects that are mounted on the wall (e.g. paintings). Don't include rugs. Only give objects that get placed onto the floor. Give no other text in the response. Only the list of objects.

**Output:**

- Sleeping:
  - Nightstand, 0.5m x 0.4m (2 items)

- Storage:
  - Dresser, 1.0m x 0.5m

- Work:
  - Desk Chair, 0.6m x 0.6m

# Primary Objects, Secondary Objects Constraints

**Prompt1**: For each of these objects: primary_objects, tell me all of the considerations and constraints for its placement within the room described as “a bedroom that is 4m x 5m”, with size: 4m x 5m that depend only on fixed features in the room like walls, windows, doors, sockets, etc. and return these as a bullet list for each object. Include practical things like whether it should be against a wall, or which side should be accessible for use (most objects will need an accessible constraint e.g. front of wardrobe needs to be accessible - however very few objects need all of their sides to be accessible and very few need their back to be accessible.) or if its tall, maybe it shouldn't block a window, etc. Bear in mind the size of the room, for example if the room is large, then the front, left, and right of the bed should be accessible, but if the room is very small, maybe only one side of the bed needs to be accessible. Only give these constraints and considerations, no other information.

**Output:**

### Bed (1.5m x 2m)
- Should be placed against a wall to maximize space.
- Should not block access to windows.
- Should not block access to doors.
- Front side should be accessible.
- Should allow for at least 60 cm of free space on one side for ease of getting in and out.
- Avoid placing under low-hanging fixtures if the ceiling is not uniformly high.

### Wardrobe (1.2m x 0.6m)
- Should be placed against a wall for stability.
- Should not block access to windows.
- Should not block access to doors.
- Front side should be accessible for opening doors/drawers.
- Avoid placing it where it will block electrical sockets, unless not in use.

- Ideally placed in a corner to save space.

### Desk (1.2m x 0.6m)
- Should be placed against a wall to maximize space.
- Should not block access to windows to ensure sufficient natural light.
- Should not block access to doors.
- Front side should be accessible for seating and working.
- Ideally positioned near electrical sockets for easy access to power supply.
- Should not block airflow from vents or radiators if present.

**Prompt 2:** Tell me all of the constraints and considerations between the objects in this list, primary_objects, that depend only on each other. These objects are for different regions, so the constraints should only really be about them being away from each other or near each other, nothing more specific. For example, maybe a desk should not be close to a bed, etc. The room is described as "a bedroom that is 4m x 5m", with size 4m x 5m. Only give the constraints and considerations between objects, no other information.

**Output:**

1. The bed should not be close to the desk.
2. The bed should not be close to the wardrobe.
3. The desk should have enough space around it to allow for comfortable work.
4. The wardrobe should be accessible without obstruction by the bed or desk.
5. Ensure there is sufficient walking space between the bed, desk, and wardrobe.

**Prompt 3:**

For each of these objects, secondary_objects, tell me all of the considerations and constraints for its placement within the room that depends only on fixed features in the room like walls, windows, doors, sockets, etc. (return these as a bullet list for each object). Include practical things like whether it should be against a wall and what side of the object (one of: left, right, back, front) or if it should be against a wall, or which side should be accessible for use (Most objects will have an accessible constraint - this would be something like the wardrobe needs to be accessible from the front so that the doors can open, or the bed needs to be accessible from the sides - but only give necessary accessible constraints. If an object can have its side against something, then don't say its side needs to be accessible e.g. for a nightstand, etc). The room is described as “a bedroom that is 4m x 5m”. Don't include any constraints that depend on other objects. Only give these constraints and considerations, no other information.

**Output:**

### Sleeping:
#### Nightstand (0.5m x 0.4m) (2 items)
- Can be placed against a wall.

### Storage:
#### Dresser (1.0m x 0.5m)
- Should be placed against a wall.
- Front should be accessible for use.

### Work:
#### Desk Chair (0.6m x 0.6m)
- Should not block any doors or windows.
- Should be near a wall socket for power if needed (e.g., for a computer).
- Should have enough space around it to pull out and sit down (at least 0.6m of free space in front).

**Prompt 4:**

Tell me all of the constraints and considerations between the objects in this list, secondary_obects, as well as in this list primary_objects. For example, a desk chair should have its front against the front of the desk, or the left side of one of the nightstands should be against the right side of the bed, etc.  Be specific with relationships between objects to include sides (one of: left, right, back, front) if appropriate, or minimum/maximum distances between objects etc. The room is described as "a bedroom that is 4m x 5m". Only give the constraints and considerations between objects, no other information.

**Output:**

1. **Bed and Nightstands:**
   - The left side of one nightstand should be against the right side of the bed.
   - The right side of the other nightstand should be against the left side of the bed.
   - The nightstands should be positioned so they are aligned with the headboard of the bed.

2. **Desk Chair and Desk:**
   - The front of the desk chair should be against the front of the desk.
   - Ensure there is adequate space behind the desk chair for movement (minimum of 0.5m).

3. **Dresser and Wardrobe:**
   - The dresser and wardrobe should be positioned in a way that allows for ease of access.
   - Maintain at least 0.5m of space in front of both the dresser and wardrobe for access.
   - The dresser and wardrobe should not be placed next to each other to avoid crowding.

4. **Bed and Dresser:**
   - Maintain a minimum distance of 0.5m between the bed and the dresser for ease of movement and access.

5. **Bed and Wardrobe:**
   - Maintain a minimum distance of 0.5m between the bed and the wardrobe for ease of movement and access.

6. **Desk and Bed/Nightstands:**
   - The desk should be positioned so there is a minimum distance of 0.5m from the bed and nightstands to avoid obstruction.
   - The desk should be placed along a wall opposite to or adjacent to the bed to avoid obstruction.

7. **Desk and Other Storage (Dresser/Wardrobe):**
   - The desk should have a minimum distance of 0.5m from the dresser and wardrobe to allow for ease of movement and access to storage items.

**Note:** Ensure that all furniture placement considers the need for adequate circulation space and ease of access to various parts of the room.

**Prompt 5:**
Given this list of primary objects: primary_objects, and this list of secondary objects: secondary_objects, use the file attached to create the objects with the correct parameters. The room name is: room_name the region names are: regions.
The room is already set up, only add in the objects using the 'create_moving_object' function. Ensure that each objects index is unique and that the indices begin from 0. The objects should be added in the correct regions. Add in all of the primary objects first. This is the file: file_contents1. No extra text, only the function calls. Don't have 'python' at the start of the code. Do not define ANY functions, only call them.

**Output:**

create_moving_object(room_name, 'bed', 1.5, 2.0, 'sleeping', 0)
create_moving_object(room_name 'wardrobe', 1.2, 0.6, 'storage', 1)
create_moving_object(room_name, 'desk', 1.2, 0.6, 'work', 2)
create_moving_object(room_name , 'nightstand', 0.5, 0.4, 'sleeping', 3)
create_moving_object(room_name , 'nightstand', 0.5, 0.4, 'sleeping', 4)
create_moving_object(room_name , 'dresser', 1.0, 0.5, 'storage', 5)
create_moving_object(room_name , 'desk chair', 0.6, 0.6, 'work', 6)

# Tertiary Objects + Positioning

**Prompt 1**: Given a room described as: "a bedroom that is 4m x 5m", with size: 4m x 5m, with these regions within it: regions, and these objects already in it: primary_objects + secondary_objects, suggest any rugs, other decorations or objects (these are things that go on top of other objects) that should be placed in the room. For example, a tv to go on the tv unit, a painting above the bed, a table lamp on the nightstand, a chandelier over the dining table, a computer to go on the desk, etc. Don't give any furniture or objects that go on the floor (other than rugs). Everything should either go on the wall, on the ceiling, or on top of a piece of furniture. Don't include curtains. Tell me the dimensions of the objects (width and length not height - in meters). If it is a wall object, its length should be 0.1m. Tell me how they should be placed (with respect to one object. e.g. painting should be placed near the dining table or lamp should be placed on a nightstand). Don't give too many objects and don't include multi-object objects e.g. gallery walls or shelves.

**Output:**
Certainly! Here are a few additions that can enhance the room, along with their dimensions and placement suggestions:

### Sleeping Area:
1. **Table Lamp**
   - **Dimensions**: 0.3m x 0.3m
   - **Placement**: One on each nightstand.

2. **Painting**
   - **Dimensions**: 1.0m x 0.1m
   - **Placement**: Centered above the bed

### Storage Area:
3. **Mirror**
   - **Dimensions**: 1.2m x 0.1m
   - **Placement**: Hang it above the dresser.

### Work Area:
4. **Desk Organizer**
   - **Dimensions**: 0.4m x 0.2m
   - **Placement**: On the desk for holding pens, papers, etc.

5. **Computer Monitor**
   - **Dimensions**: 0.5m x 0.2m
   - **Placement**: Centered on the desk.

### General Decorations:
6. **Chandelier**
   - **Dimensions**: (Round) 0.8m diameter (Height should be adjusted according to ceiling height)
   - **Placement**: Centered in the room.

7. **Rug**
   - **Dimensions**: 2.0m x 3.0m
   - **Placement**: Under the bed, extending outward to provide a soft landing spot for feet.

These additions will make the room more functional and aesthetically pleasing without overcrowding it.

**Prompt 2:**

Given this list of tertiary objects: tertiary_objects, use the function attached to create the objects with the correct parameters. The room name is: room_name. The room description is: “a bedroom that is 4m x 5m”. The room is already set up, only add in the objects using the 'create_tertiary_object' function. Ensure that each objects index is unique and that the indices begin from 0. The object names should be simple and short. The objects should be given the correct tertiary type (ceiling, floor, wall, or table). Wall objects should all have length 0.1m. Ensure that the parameters are set correctly. This is the function:

```
""""
def create_tertiary_object(room, name, width, length, tertiary, index):
        " A function that creates and places a tertiary object
        Inputs:
        room: Room for the object to be put in
        name: str, name of the object all lowercase. E.g. 'painting'
        width: float, width of the object (m)
        length: float, length of the object (m)
        tertiary: str, tertiary object type, one of "wall" (for objects that go on the wall e.g.
painting),
```

"floor" (for objects that go on the floor e.g. rug), "ceiling" (for objects that go on the ceiling e.g. chandelier),
"table" (for objects that go on a surface e.g. lamp).
index: int, index of the object in the room's tertiary object list
" """
No extra text, only the function calls. Don't have 'python' at the start of the code. Do not define ANY functions, only call them.

**Output:**

create_tertiary_object(room_name 'lamp', 0.3, 0.3, 'table', 0)
create_tertiary_object(room_name 'lamp', 0.3, 0.3, 'table', 1)
create_tertiary_object(room_name 'painting', 1.0, 0.1, 'wall', 2)
create_tertiary_object(room_name 'mirror', 1.2, 0.1, 'wall', 3)
create_tertiary_object(room_name, 'organizer', 0.4, 0.2, 'table', 4)
create_tertiary_object(room_name, 'monitor', 0.5, 0.2, 'table', 5)
create_tertiary_object(room_name, 'chandelier', 0.8, 0.8, 'ceiling', 6)
create_tertiary_object(room_name, 'rug', 2.0, 3.0, 'floor', 7)

# Style

**Prompt:**
Given the description of the room: " a bedroom that is 4m x 5m ", with size: 4m x 5m, with these objects within it: primary_objects + secondary_objects + tertiary_objects, tell me the colours of the walls and whether there should be wallpaper/paint/some other wall material. Tell me the style and colour of the windows and doors. Tell me the material and colour of the floor, and for each object, one by one, describe its colour, style, material etc. Make sure that all of the objects are cohesive together and match the description of the room.

**Output:**

Based on the dimensions provided (4m x 5m) and the list of objects, we'll create a cohesive and aesthetically pleasing bedroom design with thoughtful selections for wall treatments, flooring, and each object.

### Walls:
- **Colour:** A soft, neutral palette such as light grey or warm beige to provide a serene and relaxing environment.
- **Treatment:** High-quality paint for a clean, modern look. Avoid wallpaper to maintain simplicity and versatility.

### Floor:
- **Material:** Hardwood for durability and elegance.
- **Colour:** A medium oak finish that provides warmth and complements the neutral wall colour.

## Door:
- **Colour**: A matching dark walnut finish, consistent with the bed frame and nightstands.

- **Material**: Solid wood for durability and a high-quality feel.
- **Style**: Modern with a clean, flat panel design, featuring sleek silver hardware that ties in with the wardrobe handles. The door should maintain simplicity to blend seamlessly with the room’s overall aesthetic.

## Windows:
- **Colour and Material**::Aluminum or wood, finished in a white or light grey to match the Scandinavian-inspired wardrobe and dresser.
- **Style**: Casement windows with clear glass, providing a modern, sleek appearance while also offering excellent insulation.
---

### Objects:

1. **Bed:**
   - **Size:** Queen-sized for proportionate fitting in the room.
   - **Colour:** Dark walnut frame with a soft grey upholstered headboard.
   - **Style:** Modern with clean lines and minimalistic design.

2. **Wardrobe:**
   - **Colour:** White with sleek silver handles.
   - **Style:** Scandinavian-inspired with a focus on functionality and simplicity.

3. **Desk:**
   - **Colour:** Light wood top with white metal legs.
   - **Style:** Minimalist, providing a clutter-free workspace.

4. **Nightstands (2):**
   - **Colour:** Matching the bed frame, dark walnut.
   - **Style:** Modern with a single drawer for a clean appearance.

5. **Dresser:**
   - **Colour:** White to match the wardrobe.
   - **Style:** Contemporary with straight lines and silver handles.

6. **Desk Chair:**
   - **Colour:** Light grey fabric with a chrome base.
   - **Style:** Ergonomic and modern.

7. **Lamp (2):**
   - **Colour:** White ceramic base with a light grey shade.
   - **Style:** Elegant and simple, fitting well with nightstands and dresser.

8. **Painting:**
   - **Colour:** A modern abstract piece with predominant shades of grey, blue, and white to add a pop of colour.
   - **Style:** Framed in a sleek black frame for a gallery-quality look.

9. **Mirror:**
   - **Colour:** Frameless or with a thin silver frame.

  - **Style:** Large and full-length for functionality and room enlargement effect.

10. **Organizer:**
   - **Colour:** Soft beige fabric bins with white wooden frame.
   - **Style:** Practical and minimalistic.

11. **Monitor:**
   - **Colour:** Black.
   - **Style:** Sleek and modern, with a small footprint on the desk.

12. **Chandelier:**
   - **Colour:** Polished chrome with clear crystal accents.
   - **Style:** Modern and elegant, adding a touch of luxury to the room.

13. **Rug:**
   - **Colour:** Light grey with subtle geometric patterns in white.
   - **Style:** Plush and cozy, placed under the bed extending slightly beyond it.

---

### Cohesion and Harmony:
The selections ensure a cohesive design that blends modern, minimalistic, and Scandinavian elements. The soft neutral walls and medium oak flooring create a warm and balanced foundation. Each piece of furniture and accessory has been chosen for its simplicity, elegance, and ability to create a tranquil, aesthetically pleasing bedroom.

# Constraint Cleaning

This prompt is used 4 times:  for the primary individual constraints, for the primary inter-object constraints, for the secondary individual constraints, and the secondary inter-object constraints.

**Prompt 1**: I am going to give you a list of constraints. I want you to merge any similar constraints and also remove any duplicate constraints. Each constraint should be simplified, so that it is said in the most basic terms. I want you to remove any constraints that are contradictory e.g. should be near a window AND should be away from a window. If there is an "or" statement in the constraint, choose one of the options. Finally, each bullet constraint should only specify one constraint. For example if there is a bullet point that says and object should not block windows and doors, change this into 2 bullets - one for blocking doors, and one for blocking windows. Remove any constraints that have if statements, and any that involve height. If there are constraints for objects to be accessible from all sides that are unnecessary, change them to be which sides you think ARE necessary. If there are constraints with "or" in them, choose between the options. Return the list of cleaned constraints. Here is the list of constraints: constraints.

**Output 1:**

### Cleaned Constraints:

#### Bed (1.5m x 2m)
- Should be placed against a wall.
- Should not block access to windows.
- Should not block access to doors.
- Front side should be accessible.
- Should allow for at least 60 cm of free space on one side.

#### Wardrobe (1.2m x 0.6m)
- Should be placed against a wall.
- Should not block access to windows.
- Should not block access to doors.
- Front side should be accessible.
- Avoid placing it where it will block electrical sockets.
- Ideally placed in a corner.

#### Desk (1.2m x 0.6m)
- Should be placed against a wall.
- Should not block access to windows.
- Should not block access to doors.
- Front side should be accessible.
- Ideally positioned near electrical sockets.
- Should not block airflow from vents.

**Output 2:**

Here are the cleaned and simplified constraints based on your requirements:

- The bed should not be close to the desk.
- The bed should not be close to the wardrobe.
- The desk should have enough space around it to allow for comfortable work.
- The wardrobe should be accessible without obstruction by the bed.
- The wardrobe should be accessible without obstruction by the desk.
- Ensure there is sufficient walking space between the bed and the desk.
- Ensure there is sufficient walking space between the bed and the wardrobe.
- Ensure there is sufficient walking space between the desk and the wardrobe.

**Output 3:**

Here is the cleaned list of constraints:

### Sleeping:
#### Nightstand (0.5m x 0.4m) (2 items)
- Can be placed against a wall.

### Storage:
#### Dresser (1.0m x 0.5m)
- Should be placed against a wall.
- Front should be accessible for use.

### Work:
#### Desk Chair (0.6m x 0.6m)
- Should not block any doors.
- Should not block any windows.
- Should have enough space around it to pull out and sit down.

**Output 4:**

**Cleaned Constraints:**

1. **Bed and Nightstands:**
   - One nightstand should be to the right of the bed.
   - One nightstand should be to the left of the bed.
   - The nightstands should be aligned with the headboard of the bed.

2. **Desk Chair and Desk:**
   - The front of the desk chair should be against the front of the desk.
   - Ensure there is adequate space behind the desk chair for movement.

3. **Dresser and Wardrobe:**
   - Maintain at least 0.5m of space in front of the dresser for access.
   - Maintain at least 0.5m of space in front of the wardrobe for access.
   - The dresser and wardrobe should not be placed next to each other to avoid crowding.

4. **Bed and Dresser:**
   - Maintain a minimum distance of 0.5m between the bed and the dresser for ease of movement.

5. **Bed and Wardrobe:**
   - Maintain a minimum distance of 0.5m between the bed and the wardrobe for ease of movement.

6. **Desk and Bed/Nightstands:**
   - The desk should be positioned so there is a minimum distance of 0.5m from the bed and nightstands.
   - The desk should be placed along a wall opposite the bed.

7. **Desk and Other Storage (Dresser/Wardrobe):**
   - The desk should have a minimum distance of 0.5m from the dresser.
   - The desk should have a minimum distance of 0.5m from the wardrobe.

**General Note:** Ensure that all furniture placement considers the need for adequate circulation space and ease of access to various parts of the room.

# Translation

**Prompt 1:**

Given the room_name room_name, as well as the primary objects: primary_objects, their indices primary_indices, and these constraints: primary_individual_cons, using the script attached, transform each constraint into a SINGLE function call that will ensure that the primary objects are set up correctly. Match each constraint to the closest function in the script file by using the docstrings. Ensure that every constraint is mapped to a function call, unless there is not one that matches. Here is the first script: file_contents2. For the second script, I want you to transform each pairwise constraint into a function call. Here is the second script: file_contents3, and here is the list of pairwise constraints: primary_io_cons. I want the output to begin with: def optimize_primary_objects(positions, room): \n output = 0, followed by each constraint function call added to the output, and then the output returned (everyline should begin with 'output +=' except for the final line). Go object by object, and then pairwise. No extra text please, only the functions and the output. If there is only 1 primary object, there should be no pairwise calls. Do not define ANY functions, only call them. ENSURE that all parameters match docstrings.

**Output:**

```
def optimize_primary_objects(positions, room):
    output = 0
    output  += check_and_call('ind_next_to_wall', positions, room, 0)
    output  += check_and_call('ind_not_block_fixed_object', positions, room, 0, 'window')
    output  += check_and_call('ind_not_block_fixed_object', positions, room, 0, 'door')
    output  += check_and_call('ind_accessible', positions, room, 0, ['front'])
    output  += check_and_call('ind_accessible', positions, room, 0, ['left', 'right'], 0.6)
    output  += check_and_call('ind_next_to_wall', positions, room, 1)
    output  += check_and_call('ind_not_block_fixed_object', positions, room, 1, 'window')
    output  += check_and_call('ind_not_block_fixed_object', positions, room, 1, 'door')
    output  += check_and_call('ind_accessible', positions, room, 1, ['front'])
    output  += check_and_call('ind_away_from_fixed_object', positions, room, 1, 'socket')
    output  += check_and_call('ind_in_corner', positions, room, 1)
    output  += check_and_call('ind_next_to_wall', positions, room, 2)
    output  += check_and_call('ind_not_block_fixed_object', positions, room, 2, 'window')
    output  += check_and_call('ind_not_block_fixed_object', positions, room, 2, 'door')
    output  += check_and_call('ind_accessible', positions, room, 2, ['front'])
    output  += check_and_call('ind_close_to_fixed_object', positions, room, 2, 'socket')
    output  += check_and_call('ind_away_from_fixed_object', positions, room, 2, 'vent')
    output  += check_and_call('io_away_from', positions, room, 0, 2, 2.0)
    output  += check_and_call('io_away_from', positions, room, 0, 1, 2.0)
    output  += check_and_call('io_away_from', positions, room, 2, 1, 2.0)
    output  += check_and_call('io_away_from', positions, room, 1, 0, 2.0)
    output  += check_and_call('io_next_to', positions, room, 1, 0)
    output  += check_and_call('io_near', positions, room, 2, 0, 3.0)
    output  += check_and_call('io_near', positions, room, 1, 2, 3.0)


    output += wall_attraction(positions, room)
    output += in_bounds(positions, room)
    output += no_overlap(positions, room)
    output += aligned(positions, room)
    output += balanced(positions, room)
    return output
```

**Prompt 2:**

Given the primary objects: primary_objects, and their indices: primary_indices, as well as the secondary objects, along with their indices and their regions: [(s_i, ind_i, r_i), ..], their individual constraints: secondary_ind_cons, and the region names: regions. Using the script attached, transform each constraint into a SINGLE function call that will ensure that the secondary objects are set up correctly. Match each constraint to the closest function in the script file by using the docstrings. Ensure that every constraint is mapped to a function call, unless there is not one that fits. Here is the first script: file_contents2. For the second script, I want you to transform each pairwise constraint into a SINGLE function call. Here is the second script: file_contents3, and here is the list of pairwise constraints: s_io_cons. I want the output to begin with: ‘def optimize_secondary_objects(positions, room): \n output = 0\n’, followed by each constraint function call added to the output, (each line should begin with 'output +='). Go object by object, and then pairwise. Also ensure to use ind_in_region for each object. Do not define ANY functions, only call them. No extra text please, only the functions and the output.

**Output:**

```
def optimize_secondary_objects(positions, room):
    output = 0


    output  += check_and_call('ind_in_region', positions, room, 3, 'sleeping')
    output  += check_and_call('ind_next_to_wall', positions, room, 3)
    output  += check_and_call('ind_in_region', positions, room, 4, 'sleeping')
    output  += check_and_call('ind_next_to_wall', positions, room, 4)
    output  += check_and_call('ind_in_region', positions, room, 5, 'storage')
    output  += check_and_call('ind_next_to_wall', positions, room, 5)
    output  += check_and_call('ind_accessible', positions, room, 5, ['front'], min_dist = 0.5)
    output  += check_and_call('ind_in_region', positions, room, 6, 'work')
    output  += check_and_call('ind_not_block_fixed_object', positions, room, 6, 'door')
    output  += check_and_call('ind_not_block_fixed_object', positions, room, 6, 'window')
    output  += check_and_call('ind_accessible', positions, room, 6, ['front', 'back'], min_dist =
0.6)
    output  += check_and_call('io_next_to', positions, room, 3, 0, side1='right')
    output  += check_and_call('io_next_to', positions, room, 4, 0, side1='left')
```

```
output  += check_and_call('io_parallel', positions, room, 3, 4, max_dist=0.5)
output  += check_and_call('io_next_to', positions, room, 6, 2, side1='front', side2='front')
output  += check_and_call('ind_accessible', positions, room, 6, ['back'], min_dist=0.6)
output  += check_and_call('ind_accessible', positions, room, 5, ['front'], min_dist=0.5)
output  += check_and_call('ind_accessible', positions, room, 1, ['front'], min_dist=0.5)
output  += check_and_call('io_away_from', positions, room, 5, 1, min_dist=0.5)
output  += check_and_call('io_away_from', positions, room, 5, 0, min_dist=0.5)
output  += check_and_call('io_away_from', positions, room, 1, 0, min_dist=0.5)
output  += check_and_call('io_away_from', positions, room, 2, 0, min_dist=0.5)
output  += check_and_call('io_away_from', positions, room, 2, 4, min_dist=0.5)
output  += check_and_call('ind_next_to_wall', positions, room, 2)
output  += check_and_call('io_away_from', positions, room, 2, 5, min_dist=0.5)
output  += check_and_call('io_away_from', positions, room, 2, 1, min_dist=0.5)


output += wall_attraction(positions, room)
output += in_bounds(positions, room)
output += no_overlap(positions, room)
output += aligned(positions, room)
return output
```

**Prompt 3:**

Given all the objects in the room: primary_objects + secondary_objects,  and their indices: primary_indices + secondary_indices, as well as the region names:  regions, here are the tertiary objects and how they should be placed: tertiary_output. These are there indices: tertiary_indices. Using the script attached, transform each placement into a SINGLE function call that will ensure that the tertiary objects are placed correctly. If there is not a function that fits, then choose another. Here is the  script: file_contents4. I want the output to begin with: ‘def optimize_tertiary_objects(positions, room): \n output = 0\n’, followed by each function call added to the output, (each line should begin with 'output +='). Do not define ANY functions, only call them. No extra text please, only the functions and the output.

**Output:**

```
def optimize_tertiary_objects(positions, room):
    output = 0

    output  += check_and_call('on_top_central', positions, room, 0, 3)
    output  += check_and_call('on_top_central', positions, room, 1, 4)
    output  += check_and_call('on_wall_above_central', positions, room, 2, 0)
    output  += check_and_call('on_wall_above_central', positions, room, 3, 5)
    output  += check_and_call('on_top_central', positions, room, 4, 2)
    output  += check_and_call('on_top_central', positions, room, 5, 2)
    output  += check_and_call('center_ceiling', positions, room, 6)
    output  += check_and_call('rug_under_central_forward', positions, room, 7, 0)

    output  += check_and_call('t_valid', positions, room)
    return output
```
