# Supplementary material for: FlairGPT: Repurposing LLMs for Interior Designs
Source: arXiv:2501.04648 source file (2025-08-30)
Supplement: Supplementary file 3 [file us2.pdf]

| | | | | | | | | | | | | | | | | | |
|---|---|---|---|---|---|---|---|---|---|---|---|---|---|---|---|---|---|
| (a) Object Type<br>Ignoring the style, placement, shape, and size of the objects, please consider the type (e.g. bed or desk) of each object in the room. How much do you agree with this statement:<br>“Given the description of the room, each object in the room should be there, and there are no objects in the room that should not be there.” | 4 | 4 | 4 | 3 | 4 | 4 | 4 | 4 | 5 | 3 | 4 | 4 | 4 | 4 | 2 | 2 | 3 |
| (b) Object Size<br>Ignoring the type, style, functionality, and placement of the objects, please consider the size of each object. How much do you agree with this statement:<br>“The objects in the room are the correct size and in proportion.” | 5 | 2 | 3 | 2 | 4 | 2 | 3 | 4 | 4 | 3 | 5 | 1 | 4 | 2 | 4 | 4 | 3 |
| (c) Object Style<br>Ignoring the type, size, functionality and placement of the objects, please consider the style (colour, material, overall style e.g minimalist) of each object in the room. How much do you agree with this sta<br>“The style of the objects in the room is cohesive and matches the room description well.” | 4 | 5 | 4 | 3 | 3 | 4 | 2 | 4 | 1 | 4 | 4 | 4 | 5 | 5 | 3 | 3 | 5 |
| (d) Object Functionality<br>Ignoring the type, size, style and placement, please consider the functionality of all the objects in the room. Can the wardrobe doors open? Can you walk to the sofa and sit down?<br>How much do you agree with the following statement:<br>"I am able to easily use every object in the room." | 3 | 2 | 4 | 4 | 5 | 3 | 5 | 4 | 3 | 3 | 3 | 2 | 5 | 3 | 4 | 3 | 3 |
| (e) Object Placement<br>Ignoring the type, size, style, and functionality of the objects, please consider the placement of all the objects in the room. How much do you agree with the following statement:<br>“The room is laid out well and the objects are placed in a way that makes sense.” | 3 | 2 | 2 | 2 | 4 | 3 | 4 | 4 | 2 | 3 | 4 | 1 | 3 | 4 | 2 | 3 | 4 |
| (a) Object Type<br>Ignoring the style, placement, shape, and size of the objects, please consider the type (e.g. bed or desk) of each object in the room. How much do you agree with this statement:<br>“Given the description of the room, each object in the room should be there, and there are no objects in the room that should not be there.” | 5 | 5 | 5 | 5 | 5 | 5 | 4 | 4 | 5 | 4 | 5 | 5 | 4 | 5 | 4 | 4 | 4 |
| (b) Object Size<br>Ignoring the type, style, functionality, and placement of the objects, please consider the size of each object. How much do you agree with this statement:<br>“The objects in the room are the correct size and in proportion.” | 5 | 5 | 3 | 4 | 5 | 5 | 2 | 4 | 5 | 5 | 4 | 5 | 5 | 5 | 4 | 4 | 5 |
| (c) Object Style<br>Ignoring the type, size, functionality and placement of the objects, please consider the style (colour, material, overall style e.g minimalist) of each object in the room. How much do you agree with this sta<br>“The style of the objects in the room is cohesive and matches the room description well.” | 4 | 5 | 4 | 5 | 4 | 4 | 2 | 4 | 4 | 5 | 4 | 5 | 5 | 5 | 5 | 4 | 3 |
| (d) Object Functionality<br>Ignoring the type, size, style and placement, please consider the functionality of all the objects in the room. Can the wardrobe doors open? Can you walk to the sofa and sit down?<br>How much do you agree with the following statement:<br>"I am able to easily use every object in the room." | 3 | 4 | 4 | 4 | 5 | 2 | 2 | 2 | 2 | 5 | 5 | 4 | 5 | 5 | 4 | 4 | 5 |
| (e) Object Placement<br>Ignoring the type, size, style, and functionality of the objects, please consider the placement of all the objects in the room. How much do you agree with the following statement:<br>“The room is laid out well and the objects are placed in a way that makes sense.” | 4 | 4 | 3 | 5 | 4 | 2 | 4 | 2 | 2 | 4 | 3 | 4 | 4 | 4 | 3 | 3 | 5 |
| (a) Object Type<br>Ignoring the style, placement, shape, and size of the objects, please consider the type (e.g. bed or desk) of each object in the room. How much do you agree with this statement:<br>“Given the description of the room, each object in the room should be there, and there are no objects in the room that should not be there.” | 4 | 4 | 4 | 3 | 4 | 3 | 4 | 4 | 2 | 4 | 5 | 3 | 4 | 5 | 3 | 4 | 4 |
| (b) Object Size<br>Ignoring the type, style, functionality, and placement of the objects, please consider the size of each object. How much do you agree with this statement:<br>“The objects in the room are the correct size and in proportion.” | 4 | 5 | 3 | 4 | 4 | 5 | 4 | 3 | 2 | 5 | 4 | 4 | 5 | 4 | 4 | 4 | 4 |
| (c) Object Style<br>Ignoring the type, size, functionality and placement of the objects, please consider the style (colour, material, overall style e.g minimalist) of each object in the room. How much do you agree with this sta<br>“The style of the objects in the room is cohesive and matches the room description well.” | 5 | 5 | 4 | 3 | 4 | 5 | 4 | 4 | 4 | 5 | 4 | 4 | 5 | 5 | 5 | 4 | 5 |
| (d) Object Functionality<br>Ignoring the type, size, style and placement, please consider the functionality of all the objects in the room. Can the wardrobe doors open? Can you walk to the sofa and sit down?<br>How much do you agree with the following statement:<br>"I am able to easily use every object in the room." | 4 | 5 | 4 | 2 | 5 | 4 | 4 | 4 | 4 | 5 | 4 | 5 | 5 | 5 | 5 | 5 | 5 |
| (e) Object Placement<br>Ignoring the type, size, style, and functionality of the objects, please consider the placement of all the objects in the room. How much do you agree with the following statement:<br>“The room is laid out well and the objects are placed in a way that makes sense.” | 4 | 4 | 3 | 1 | 4 | 3 | 4 | 3 | 3 | 4 | 5 | 3 | 4 | 3 | 3 | 4 | 2 |
| (a) Object Type<br>Ignoring the style, placement, shape, and size of the objects, please consider the type (e.g. bed or desk) of each object in the room. How much do you agree with this statement:<br>“Given the description of the room, each object in the room should be there, and there are no objects in the room that should not be there.” | 4 | 5 | 4 | 5 | 5 | 3 | 4 | 3 | 4 | 5 | 5 | 5 | 5 | 5 | 4 | 5 | 5 |
| (b) Object Size<br>Ignoring the type, style, functionality, and placement of the objects, please consider the size of each object. How much do you agree with this statement:<br>“The objects in the room are the correct size and in proportion.” | 5 | 5 | 5 | 5 | 5 | 3 | 4 | 4 | 5 | 5 | 5 | 5 | 5 | 5 | 5 | 5 | 4 |
| (c) Object Style<br>Ignoring the type, size, functionality and placement of the objects, please consider the style (colour, material, overall style e.g minimalist) of each object in the room. How much do you agree with this sta<br>“The style of the objects in the room is cohesive and matches the room description well.” | 4 | 5 | 5 | 5 | 5 | 4 | 2 | 4 | 4 | 5 | 4 | 5 | 5 | 5 | 3 | 5 | 4 |
| (d) Object Functionality<br>Ignoring the type, size, style and placement, please consider the functionality of all the objects in the room. Can the wardrobe doors open? Can you walk to the sofa and sit down?<br>How much do you agree with the following statement:<br>"I am able to easily use every object in the room." | 4 | 5 | 4 | 5 | 5 | 5 | 5 | 3 | 4 | 5 | 5 | 5 | 5 | 5 | 5 | 5 | 4 |
| (e) Object Placement<br>Ignoring the type, size, style, and functionality of the objects, please consider the placement of all the objects in the room. How much do you agree with the following statement:<br>“The room is laid out well and the objects are placed in a way that makes sense.” | 3 | 4 | 4 | 5 | 5 | 5 | 5 | 4 | 4 | 5 | 5 | 5 | 5 | 5 | 4 | 5 | 4 |
| (a) Object Type<br>Ignoring the style, placement, shape, and size of the objects, please consider the type (e.g. bed or desk) of each object in the room. How much do you agree with this statement:<br>“Given the description of the room, each object in the room should be there, and there are no objects in the room that should not be there.” | 4 | 5 | 5 | 4 | 5 | 5 | 3 | 4 | 5 | 4 | 4 | 5 | 5 | 4 | 5 | 3 | 4 |
| (b) Object Size<br>Ignoring the type, style, functionality, and placement of the objects, please consider the size of each object. How much do you agree with this statement:<br>“The objects in the room are the correct size and in proportion.” | 4 | 5 | 4 | 4 | 5 | 5 | 4 | 3 | 4 | 3 | 4 | 5 | 5 | 5 | 5 | 4 | 5 |
| (c) Object Style<br>Ignoring the type, size, functionality and placement of the objects, please consider the style (colour, material, overall style e.g minimalist) of each object in the room. How much do you agree with this sta<br>“The style of the objects in the room is cohesive and matches the room description well.” | 4 | 5 | 4 | 4 | 5 | 5 | 5 | 4 | 4 | 2 | 3 | 4 | 5 | 5 | 3 | 4 | 5 |
| (d) Object Functionality<br>Ignoring the type, size, style and placement, please consider the functionality of all the objects in the room. Can the wardrobe doors open? Can you walk to the sofa and sit down?<br>How much do you agree with the following statement:<br>"I am able to easily use every object in the room." | 4 | 4 | 4 | 4 | 5 | 3 | 5 | 4 | 5 | 2 | 4 | 5 | 5 | 3 | 5 | 3 | 4 |
| (e) Object Placement<br>Ignoring the type, size, style, and functionality of the objects, please consider the placement of all the objects in the room. How much do you agree with the following statement:<br>“The room is laid out well and the objects are placed in a way that makes sense.” | 3 | 2 | 3 | 4 | 5 | 2 | 4 | 3 | 2 | 2 | 3 | 3 | 5 | 4 | 4 | 3 | 4 |
| (a) Object Type<br>Ignoring the style, placement, shape, and size of the objects, please consider the type (e.g. bed or desk) of each object in the room. How much do you agree with this statement:<br>“Given the description of the room, each object in the room should be there, and there are no objects in the room that should not be there.” | 4 | 5 | 5 | 5 | 5 | 5 | 4 | 4 | 5 | 5 | 5 | 5 | 5 | 5 | 4 | 5 | 5 |
| (b) Object Size<br>Ignoring the type, style, functionality, and placement of the objects, please consider the size of each object. How much do you agree with this statement:<br>“The objects in the room are the correct size and in proportion.” | 4 | 3 | 3 | 2 | 3 | 3 | 2 | 3 | 5 | 5 | 5 | 2 | 5 | 2 | 4 | 5 | 3 |
| (c) Object Style<br>Ignoring the type, size, functionality and placement of the objects, please consider the style (colour, material, overall style e.g minimalist) of each object in the room. How much do you agree with this sta<br>“The style of the objects in the room is cohesive and matches the room description well.” | 5 | 5 | 4 | 4 | 5 | 5 | 3 | 3 | 5 | 5 | 4 | 4 | 5 | 5 | 4 | 5 | 3 |
| (d) Object Functionality<br>Ignoring the type, size, style and placement, please consider the functionality of all the objects in the room. Can the wardrobe doors open? Can you walk to the sofa and sit down?<br>How much do you agree with the following statement:<br>"I am able to easily use every object in the room." | 4 | 5 | 4 | 4 | 5 | 5 | 4 | 3 | 5 | 5 | 5 | 5 | 5 | 5 | 5 | 5 | 4 |
| (e) Object Placement<br>Ignoring the type, size, style, and functionality of the objects, please consider the placement of all the objects in the room. How much do you agree with the following statement:<br>“The room is laid out well and the objects are placed in a way that makes sense.” | 3 | 4 | 3 | 5 | 4 | 5 | 3 | 4 | 5 | 5 | 5 | 4 | 5 | 5 | 3 | 5 | 2 |
| (a) Object Type<br>Ignoring the style, placement, shape, and size of the objects, please consider the type (e.g. bed or desk) of each object in the room. How much do you agree with this statement:<br>“Given the description of the room, each object in the room should be there, and there are no objects in the room that should not be there.” | 4 | 3 | 2 | 4 | 4 | 3 | 1 | 3 | 4 | 1 | 3 | 3 | 4 | 5 | 2 | 4 | 5 |
| (b) Object Size<br>Ignoring the type, style, functionality, and placement of the objects, please consider the size of each object. How much do you agree with this statement:<br>“The objects in the room are the correct size and in proportion.” | 5 | 4 | 4 | 4 | 5 | 3 | 4 | 4 | 3 | 1 | 4 | 4 | 5 | 5 | 4 | 4 | 5 |
| (c) Object Style<br>Ignoring the type, size, functionality and placement of the objects, please consider the style (colour, material, overall style e.g minimalist) of each object in the room. How much do you agree with this sta<br>“The style of the objects in the room is cohesive and matches the room description well.” | 4 | 4 | 4 | 4 | 3 | 5 | 2 | 4 | 3 | 2 | 4 | 5 | 4 | 5 | 3 | 2 | 5 |
| (d) Object Functionality<br>Ignoring the type, size, style and placement, please consider the functionality of all the objects in the room. Can the wardrobe doors open? Can you walk to the sofa and sit down?<br>How much do you agree with the following statement:<br>"I am able to easily use every object in the room." | 4 | 5 | 4 | 5 | 5 | 5 | 3 | 3 | 2 | 2 | 5 | 5 | 5 | 5 | 5 | 4 | 5 |
| (e) Object Placement<br>Ignoring the type, size, style, and functionality of the objects, please consider the placement of all the objects in the room. How much do you agree with the following statement:<br>“The room is laid out well and the objects are placed in a way that makes sense.” | 4 | 3 | 4 | 4 | 5 | 3 | 1 | 4 | 2 | 1 | 5 | 5 | 5 | 5 | 3 | 2 | 5 |

| | | | | | | | | | | | | | | | | | |
|---|---|---|---|---|---|---|---|---|---|---|---|---|---|---|---|---|---|
| (a) Object Type<br>Ignoring the style, placement, shape, and size of the objects, please consider the type (e.g. bed or desk) of each object in the room. How much do you agree with this statement:<br>“Given the description of the room, each object in the room should be there, and there are no objects in the room that should not be there.” | 5 | 5 | 4 | 4 | 5 | 5 | 4 | 4 | 5 | 5 | 5 | 4 | 5 | 5 | 4 | 4 | 4 |
| (b) Object Size<br>Ignoring the type, style, functionality, and placement of the objects, please consider the size of each object. How much do you agree with this statement:<br>“The objects in the room are the correct size and in proportion.” | 4 | 5 | 4 | 4 | 5 | 5 | 4 | 4 | 4 | 4 | 5 | 5 | 5 | 5 | 4 | 5 | 3 |
| (c) Object Style<br>Ignoring the type, size, functionality and placement of the objects, please consider the style (colour, material, overall style e.g minimalist) of each object in the room. How much do you agree with this sta<br><br>“The style of the objects in the room is cohesive and matches the room description well.” | 5 | 5 | 5 | 5 | 4 | 5 | 5 | 4 | 5 | 4 | 5 | 5 | 5 | 5 | 4 | 5 | 4 |
| (d) Object Functionality<br><br>Ignoring the type, size, style and placement, please consider the functionality of all the objects in the room. Can the wardrobe doors open?  Can you walk to the sofa and sit down?<br><br>How much do you agree with the following statement:<br>“I am able to easily use every object in the room." | 4 | 5 | 4 | 5 | 5 | 5 | 4 | 4 | 4 | 4 | 4 | 5 | 5 | 5 | 4 | 4 | 3 |
| (e) Object Placement<br><br>Ignoring the type, size, style, and functionality of the objects, please consider the placement of all the objects in the room. How much do you agree with the following statement:<br><br>“The room is laid out well and the objects are placed in a way that makes sense.” | 4 | 5 | 3 | 5 | 5 | 5 | 4 | 4 | 3 | 5 | 4 | 4 | 5 | 4 | 4 | 4 | 4 |
| (a) Object Type<br>Ignoring the style, placement, shape, and size of the objects, please consider the type (e.g. bed or desk) of each object in the room. How much do you agree with this statement:<br>“Given the description of the room, each object in the room should be there, and there are no objects in the room that should not be there.” | 5 | 5 | 4 | 5 | 5 | 4 | 4 | 3 | 5 | 5 | 5 | 4 | 5 | 5 | 3 | 4 | 4 |
| (b) Object Size<br>Ignoring the type, style, functionality, and placement of the objects, please consider the size of each object. How much do you agree with this statement:<br>“The objects in the room are the correct size and in proportion.” | 3 | 4 | 2 | 4 | 5 | 2 | 3 | 2 | 4 | 5 | 5 | 3 | 5 | 4 | 4 | 4 | 3 |
| (c) Object Style<br>Ignoring the type, size, functionality and placement of the objects, please consider the style (colour, material, overall style e.g minimalist) of each object in the room. How much do you agree with this sta<br><br>“The style of the objects in the room is cohesive and matches the room description well.” | 4 | 5 | 4 | 5 | 5 | 5 | 4 | 3 | 5 | 4 | 4 | 5 | 5 | 5 | 4 | 5 | 4 |
| (d) Object Functionality<br><br>Ignoring the type, size, style and placement, please consider the functionality of all the objects in the room. Can the wardrobe doors open?  Can you walk to the sofa and sit down?<br><br>How much do you agree with the following statement:<br>“I am able to easily use every object in the room." | 4 | 5 | 3 | 5 | 5 | 2 | 4 | 3 | 2 | 4 | 5 | 5 | 5 | 3 | 5 | 4 | 3 |
| (e) Object Placement<br><br>Ignoring the type, size, style, and functionality of the objects, please consider the placement of all the objects in the room. How much do you agree with the following statement:<br><br>“The room is laid out well and the objects are placed in a way that makes sense.” | 4 | 4 | 3 | 5 | 5 | 3 | 4 | 3 | 2 | 5 | 5 | 4 | 5 | 3 | 3 | 4 | 3 |
